# Supplementary material for: Order-by-disorder charge density wave condensation at $\mathbf{\textit{q} =(\frac{1}{3},\frac{1}{3},\frac{1}{3})}$ in kagome metal ScV$_6$Sn$_6$
Source: arXiv:2308.11553 ancillary file (2023-08-23)
Supplement: Supplementary file 1 [file scv6sn6-paper_supp.pdf]

# Oder-by-disorder charge density wave condensation at $q = (\frac{1}{3}, \frac{1}{3}, \frac{1}{3})$ in kagome metal $ScV_6Sn_6$
# - Supplemental Material -

Alaska Subedi
*CPHT, CNRS, École polytechnique, Institut Polytechnique de Paris, 91120 Palaiseau, France*
(Dated: August 17, 2023)

Calculated lattice parameters and atomic coordinates of $ScV_6Sn_6$ for all the phases discussed in the paper are given below.

TABLE I. Parent $P6/mmm$ phase with relative energy 0 meV/f.u.
$a = b = 5.426722$ Å, $c = 9.221546$ Å, $\alpha = \beta = 90°$, $\gamma = 120°$.

| Atom | Wyckoff | $x$ | $y$ | $z$ |
|---|---|---|---|---|
| Sc1 | 1a | 0.00000 | 0.00000 | 0.00000 |
| V1 | 6i | 0.50000 | 0.00000 | 0.24771 |
| Sn1 | 2e | 0.00000 | 0.00000 | 0.68161 |
| Sn2 | 2c | 0.33333 | 0.66667 | 0.00000 |
| Sn3 | 2d | 0.33333 | 0.66667 | 0.50000 |

TABLE II. $H_3(a, 0)$ $P6/mmm$ phase with relative energy $-16.68$ meV/f.u.
$a = b = 9.396434$ Å, $c = 18.482209$ Å, $\alpha = \beta = 90°$, $\gamma = 120°$.

| Atom | Wyckoff | $x$ | $y$ | $z$ |
|---|---|---|---|---|
| Sc1 | 4h | 0.33333 | 0.66667 | 0.74084 |
| Sc2 | 2e | 0.00000 | 0.00000 | 0.75995 |
| V1 | 12o | 0.16621 | 0.33242 | 0.87401 |
| V2 | 6i | 0.50000 | 0.00000 | 0.87361 |
| V3 | 12o | 0.16714 | 0.33429 | 0.37361 |
| V4 | 6i | 0.50000 | 0.00000 | 0.37411 |
| Sn1 | 4h | 0.33333 | 0.66667 | 0.09987 |
| Sn2 | 2e | 0.00000 | 0.00000 | 0.08279 |
| Sn3 | 4h | 0.33333 | 0.66667 | 0.58353 |
| Sn4 | 2e | 0.00000 | 0.00000 | 0.60088 |
| Sn5 | 12n | 0.66657 | 0.00000 | 0.74987 |
| Sn6 | 6j | 0.66487 | 0.00000 | 0.00000 |
| Sn7 | 6k | 0.66864 | 0.00000 | 0.50000 |

TABLE III. $H_3(0, a)$ $P6_3/mmc$ phase with relative energy $-10.64$ meV/f.u.
$a = b = 9.397346$ Å, $c = 18.48375$ Å, $\alpha = \beta = 90°$, $\gamma = 120°$.

| Atom | Wyckoff | $x$ | $y$ | $z$ |
|---|---|---|---|---|
| Sc1 | 2a | 0.00000 | 0.00000 | 0.00000 |
| Sc2 | 4f | 0.33333 | 0.66667 | 0.50886 |
| V1 | 12k | 0.83315 | 0.66629 | 0.12410 |
| V2 | 12k | 0.50043 | 0.00085 | 0.12375 |
| V3 | 12k | 0.16642 | 0.33284 | 0.12367 |
| Sn1 | 4e | 0.00000 | 0.00000 | 0.34104 |
| Sn2 | 4f | 0.33333 | 0.66667 | 0.83365 |
| Sn3 | 4f | 0.33333 | 0.66667 | 0.34968 |
| Sn4 | 12i | 0.66688 | 0.00000 | 0.00000 |
| Sn5 | 12j | 0.33259 | 0.33439 | 0.25000 |

TABLE IV. $L_2^-(a, 0, 0)$ $Immm$ phase with relative energy $-12.10$ meV/f.u.
$a = 5.428245$ Å, $b = 9.391430$ Å, $c = 18.480583$ Å, $\alpha = \beta = \gamma = 90°$.

| Atom | Wyckoff | $x$ | $y$ | $z$ |
|---|---|---|---|---|
| Sc1 | 4i | 0.00000 | 0.00000 | 0.75954 |
| V1 | 16o | 0.74753 | 0.74962 | 0.37381 |
| V2 | 4j | 0.50000 | 0.00000 | 0.87437 |
| V3 | 4j | 0.50000 | 0.00000 | 0.37326 |
| Sn1 | 4i | 0.00000 | 0.00000 | 0.08311 |
| Sn2 | 4i | 0.00000 | 0.00000 | 0.60022 |
| Sn3 | 8l | 0.00000 | 0.33338 | 0.74943 |
| Sn4 | 4g | 0.00000 | 0.33558 | 0.00000 |
| Sn5 | 4h | 0.00000 | 0.33064 | 0.50000 |

TABLE V. $L_2^-(a, -a, 0)$ $Fmmm$ phase with relative energy $-4.01$ meV/f.u.
$a = 10.851374$ Å, $b = 18.454939$ Å, $c = 18.799248$ Å, $\alpha = \beta = \gamma = 90°$.

| Atom | Wyckoff | $x$ | $y$ | $z$ |
|---|---|---|---|---|
| Sc1 | 8h | 0.00000 | 0.24224 | 0.00000 |
| Sc2 | 8f | 0.25000 | 0.25000 | 0.25000 |
| V1 | 32p | 0.62517 | 0.12591 | 0.37533 |
| V2 | 32p | 0.37516 | 0.12643 | 0.12530 |
| V3 | 16o | 0.24920 | 0.12623 | 0.00000 |
| V4 | 16m | 0.00000 | 0.62610 | 0.75049 |
| Sn1 | 8h | 0.00000 | -0.08437 | 0.00000 |
| Sn2 | 16k | 0.25000 | 0.40924 | 0.25000 |
| Sn3 | 8h | 0.00000 | 0.40165 | 0.00000 |
| Sn4 | 16j | 0.25000 | 0.25000 | -0.08341 |
| Sn5 | 16m | 0.00000 | 0.74949 | 0.66674 |
| Sn6 | 16n | 0.75158 | 0.00000 | 0.41674 |
| Sn7 | 8i | 0.00000 | 0.00000 | 0.16717 |
| Sn8 | 8i | 0.00000 | 0.00000 | 0.66611 |

TABLE VI. $L_2^-(a,a,a)$ $P6/mmm$ phase with relative energy $-7.50$ meV/f.u.
$a = b = 10.851668$ Å, $c = 18.469036$ Å, $\alpha = \beta = 90°$, $\gamma = 120°$.

| Atom | Wyckoff | $x$ | $y$ | $z$ |
|---|---|---|---|---|
| Sc1 | 2e | 0.00000 | 0.00000 | 0.75886 |
| Sc2 | 6i | 0.50000 | 0.00000 | 0.74228 |
| V1 | 12n | 0.24925 | 0.00000 | 0.87416 |
| V2 | 12o | 0.25044 | 0.50088 | 0.87363 |
| V3 | 12n | 0.25086 | 0.00000 | 0.37350 |
| V4 | 12o | 0.24948 | 0.49896 | 0.37400 |
| Sn1 | 2e | 0.00000 | 0.00000 | 0.08352 |
| Sn2 | 6i | 0.50000 | 0.00000 | 0.09823 |
| Sn3 | 2e | 0.00000 | 0.00000 | 0.59966 |
| Sn4 | 6i | 0.50000 | 0.00000 | 0.58452 |
| Sn5 | 12o | 0.83333 | 0.66667 | 0.75011 |
| Sn6 | 4h | 0.33333 | 0.66667 | 0.74907 |
| Sn7 | 6l | 0.83225 | 0.66450 | 0.00000 |
| Sn8 | 2c | 0.33333 | 0.66667 | 0.00000 |
| Sn9 | 6m | 0.83445 | 0.66889 | 0.50000 |
| Sn10 | 2d | 0.33333 | 0.66667 | 0.50000 |

TABLE VII. $P_1(a,0,0,0)$ $R\bar{3}m$ phase with relative energy $-3.07$ meV/f.u.
$a = b = 9.398420$ Å, $c = 27.677000$ Å, $\alpha = \beta = 90°$, $\gamma = 120°$.

| Atom | Wyckoff | $x$ | $y$ | $z$ |
|---|---|---|---|---|
| Sc1 | 6c | 0.00000 | 0.00000 | 0.82848 |
| Sc2 | 3b | 0.00000 | 0.00000 | 0.50000 |
| V1 | 18h | 0.83377 | 0.16623 | 0.24915 |
| V2 | 18h | 0.16636 | 0.83364 | 0.24935 |
| V3 | 18h | 0.49985 | 0.50015 | 0.24913 |
| Sn1 | 6c | 0.00000 | 0.00000 | 0.06557 |
| Sn2 | 6c | 0.00000 | 0.00000 | 0.39261 |
| Sn3 | 6c | 0.00000 | 0.00000 | 0.72331 |
| Sn4 | 18g | 0.33302 | 0.00000 | 0.50000 |
| Sn5 | 18f | 0.33210 | 0.00000 | 0.00000 |

TABLE VIII. $P_1(-a,0,0,0)$ $R\bar{3}m$ phase with relative energy $-1.17$ meV/f.u.
$a = b = 9.398720$ Å, $c = 27.674654$ Å, $\alpha = \beta = 90°$, $\gamma = 120°$.

| Atom | Wyckoff | $x$ | $y$ | $z$ |
|---|---|---|---|---|
| Sc1 | 3a | 0.00000 | 0.00000 | 0.00000 |
| Sc2 | 6c | 0.00000 | 0.00000 | 0.33594 |
| V1 | 18h | 0.16673 | 0.83327 | 0.08260 |
| V2 | 18h | 0.49980 | 0.50020 | 0.08258 |
| V3 | 18h | 0.83347 | 0.16653 | 0.08250 |
| Sn1 | 6c | 0.00000 | 0.00000 | 0.22934 |
| Sn2 | 6c | 0.00000 | 0.00000 | 0.55794 |
| Sn3 | 6c | 0.00000 | 0.00000 | 0.89463 |
| Sn4 | 18f | 0.33343 | 0.00000 | 0.00000 |
| Sn5 | 18g | 0.33394 | 0.00000 | 0.50000 |

TABLE IX. $P_1(a,0,a,0)$ $P6/mmm$ phase with relative energy $-2.18$ meV/f.u.
$a = b = 9.398411$ Å, $c = 27.677876$ Å, $\alpha = \beta = 90°$, $\gamma = 120°$.

| Atom | Wyckoff | $x$ | $y$ | $z$ |
|---|---|---|---|---|
| Sc1 | 2d | 0.33333 | 0.66667 | 0.50000 |
| Sc2 | 1b | 0.00000 | 0.00000 | 0.50000 |
| Sc3 | 4h | 0.33333 | 0.66667 | 0.83630 |
| Sc4 | 2e | 0.00000 | 0.00000 | 0.82801 |
| V1 | 6i | 0.50000 | 0.00000 | 0.58252 |
| V2 | 12o | 0.16677 | 0.33354 | 0.58258 |
| V3 | 6i | 0.50000 | 0.00000 | -0.08397 |
| V4 | 12o | 0.16699 | 0.33398 | -0.08421 |
| V5 | 6i | 0.50000 | 0.00000 | 0.24915 |
| V6 | 12o | 0.16628 | 0.33255 | 0.24927 |
| Sn1 | 4h | 0.33333 | 0.66667 | 0.72968 |
| Sn2 | 2e | 0.00000 | 0.00000 | 0.72284 |
| Sn3 | 4h | 0.33333 | 0.66667 | 0.05768 |
| Sn4 | 2e | 0.00000 | 0.00000 | 0.06597 |
| Sn5 | 4h | 0.33333 | 0.66667 | 0.39477 |
| Sn6 | 2e | 0.00000 | 0.00000 | 0.39236 |
| Sn7 | 6k | 0.66697 | 0.00000 | 0.50000 |
| Sn8 | 12n | 0.66649 | 0.00000 | 0.83333 |
| Sn9 | 12n | 0.66602 | 0.00000 | 0.66667 |
| Sn10 | 6j | 0.66806 | 0.00000 | 0.00000 |

TABLE X. $P_1(-a,0,-a,0)$ $P6/mmm$ phase with relative energy $-1.76$ meV/f.u.
$a = b = 9.398474$ Å, $c = 27.677998$ Å, $\alpha = \beta = 90°$, $\gamma = 120°$.

| Atom | Wyckoff | $x$ | $y$ | $z$ |
|---|---|---|---|---|
| Sc1 | 1a | 0.00000 | 0.00000 | 0.00000 |
| Sc2 | 2c | 0.33333 | 0.66667 | 0.00000 |
| Sc3 | 2e | 0.00000 | 0.00000 | 0.33708 |
| Sc4 | 4h | 0.33333 | 0.66667 | 0.32983 |
| V1 | 12o | 0.83340 | 0.66680 | 0.08246 |
| V2 | 6i | 0.50000 | 0.00000 | 0.08254 |
| V3 | 12o | 0.83359 | 0.66718 | 0.41593 |
| V4 | 6i | 0.50000 | 0.00000 | 0.41577 |
| V5 | 12o | 0.83300 | 0.66600 | 0.74926 |
| V6 | 6i | 0.50000 | 0.00000 | 0.74939 |
| Sn1 | 2e | 0.00000 | 0.00000 | 0.23030 |
| Sn2 | 4h | 0.33333 | 0.66667 | 0.22448 |
| Sn3 | 2e | 0.00000 | 0.00000 | 0.55684 |
| Sn4 | 4h | 0.33333 | 0.66667 | 0.56420 |
| Sn5 | 2e | 0.00000 | 0.00000 | 0.89505 |
| Sn6 | 4h | 0.33333 | 0.66667 | 0.89308 |
| Sn7 | 6j | 0.33359 | 0.00000 | 0.00000 |
| Sn8 | 12n | 0.33327 | 0.00000 | 0.33322 |
| Sn9 | 12n | 0.33274 | 0.00000 | 0.16657 |
| Sn10 | 6k | 0.33442 | 0.00000 | 0.50000 |

TABLE XI. $P_1(a,b,a,b)$ $P6mm$ phase with relative energy $-2.20$ meV/fu.
$a = b = 9.398468$ Å, $c = 27.677639$ Å, $\alpha = \beta = 90°$, $\gamma = 120°$.

| Atom | Wyckoff | $x$ | $y$ | $z$ |
|---|---|---|---|---|
| Sc1 | 1a | 0.00000 | 0.00000 | -0.00519 |
| Sc2 | 2b | 0.33333 | 0.66667 | 0.00272 |
| Sc3 | 1a | 0.00000 | 0.00000 | 0.33868 |
| Sc4 | 2b | 0.33333 | 0.66667 | 0.33021 |
| Sc5 | 1a | 0.00000 | 0.00000 | 0.66649 |
| Sc6 | 2b | 0.33333 | 0.66667 | 0.66707 |
| V1 | 6e | 0.16697 | 0.83303 | 0.08244 |
| V2 | 3c | 0.50000 | 0.00000 | 0.08268 |
| V3 | 6e | 0.16627 | 0.83373 | 0.41593 |
| V4 | 3c | 0.50000 | 0.00000 | 0.41581 |
| V5 | 6e | 0.16679 | 0.83321 | 0.74926 |
| V6 | 3c | 0.50000 | 0.00000 | 0.74921 |
| V7 | 6e | 0.83300 | 0.16700 | 0.25086 |
| V8 | 3c | 0.50000 | 0.00000 | 0.25061 |
| V9 | 6e | 0.83325 | 0.16675 | 0.58409 |
| V10 | 3c | 0.50000 | 0.00000 | 0.58416 |
| V11 | 6e | 0.83372 | 0.16628 | -0.08258 |
| V12 | 3c | 0.50000 | 0.00000 | -0.08248 |
| Sn1 | 1a | 0.00000 | 0.00000 | 0.23262 |
| Sn2 | 2b | 0.33333 | 0.66667 | 0.22426 |
| Sn3 | 1a | 0.00000 | 0.00000 | 0.55889 |
| Sn4 | 2b | 0.33333 | 0.66667 | 0.56179 |
| Sn5 | 1a | 0.00000 | 0.00000 | 0.88966 |
| Sn6 | 2b | 0.33333 | 0.66667 | 0.89606 |
| Sn7 | 1a | 0.00000 | 0.00000 | 0.10077 |
| Sn8 | 2b | 0.33333 | 0.66667 | 0.10883 |
| Sn9 | 1a | 0.00000 | 0.00000 | 0.44389 |
| Sn10 | 2b | 0.33333 | 0.66667 | 0.43677 |
| Sn11 | 1a | 0.00000 | 0.00000 | 0.77414 |
| Sn12 | 2b | 0.33333 | 0.66667 | 0.77229 |
| Sn13 | 6d | 0.33352 | 0.00000 | 0.00000 |
| Sn14 | 6d | 0.33350 | 0.00000 | 0.33332 |
| Sn15 | 6d | 0.33304 | 0.00000 | 0.66669 |
| Sn16 | 6d | 0.33196 | 0.00000 | 0.16664 |
| Sn17 | 6d | 0.33403 | 0.00000 | 0.50000 |
| Sn18 | 6d | 0.33391 | 0.00000 | 0.83336 |

TABLE XII. $P_1(-a,-b,-a,-b)$ $P6mm$ phase with relative energy $-1.92$ meV/fu.
$a = b = 9.398599$ Å, $c = 27.678013$ Å, $\alpha = \beta = 90°$, $\gamma = 120°$.

| Atom | Wyckoff | $x$ | $y$ | $z$ |
|---|---|---|---|---|
| Sc1 | 1a | 0.00000 | 0.00000 | -0.00092 |
| Sc2 | 2b | 0.33333 | 0.66667 | 0.00027 |
| Sc3 | 1a | 0.00000 | 0.00000 | 0.33760 |
| Sc4 | 2b | 0.33333 | 0.66667 | 0.32976 |
| Sc5 | 1a | 0.00000 | 0.00000 | 0.66331 |
| Sc6 | 2b | 0.33333 | 0.66667 | 0.66996 |
| V1 | 6e | 0.16666 | 0.83334 | 0.08245 |
| V2 | 3c | 0.50000 | 0.00000 | 0.08256 |
| V3 | 6e | 0.16638 | 0.83362 | 0.41594 |
| V4 | 3c | 0.50000 | 0.00000 | 0.41578 |
| V5 | 6e | 0.16698 | 0.83302 | 0.74926 |
| V6 | 3c | 0.50000 | 0.00000 | 0.74937 |
| V7 | 6e | 0.83298 | 0.16702 | 0.25075 |
| V8 | 3c | 0.50000 | 0.00000 | 0.25059 |
| V9 | 6e | 0.83355 | 0.16645 | 0.58408 |
| V10 | 3c | 0.50000 | 0.00000 | 0.58423 |
| V11 | 6e | 0.83345 | 0.16655 | -0.08248 |
| V12 | 3c | 0.50000 | 0.00000 | -0.08254 |
| Sn1 | 1a | 0.00000 | 0.00000 | 0.23093 |
| Sn2 | 2b | 0.33333 | 0.66667 | 0.22436 |
| Sn3 | 1a | 0.00000 | 0.00000 | 0.55702 |
| Sn4 | 2b | 0.33333 | 0.66667 | 0.56407 |
| Sn5 | 1a | 0.00000 | 0.00000 | 0.89419 |
| Sn6 | 2b | 0.33333 | 0.66667 | 0.89334 |
| Sn7 | 1a | 0.00000 | 0.00000 | 0.10409 |
| Sn8 | 2b | 0.33333 | 0.66667 | 0.10716 |
| Sn9 | 1a | 0.00000 | 0.00000 | 0.44348 |
| Sn10 | 2b | 0.33333 | 0.66667 | 0.43580 |
| Sn11 | 1a | 0.00000 | 0.00000 | 0.77028 |
| Sn12 | 2b | 0.33333 | 0.66667 | 0.77528 |
| Sn13 | 6d | 0.33359 | 0.00000 | 0.00000 |
| Sn14 | 6d | 0.33332 | 0.00000 | 0.33323 |
| Sn15 | 6d | 0.33324 | 0.00000 | 0.66678 |
| Sn16 | 6d | 0.33259 | 0.00000 | 0.16657 |
| Sn17 | 6d | 0.33441 | 0.00000 | 0.50000 |
| Sn18 | 6d | 0.33288 | 0.00000 | 0.83342 |
